# Supplementary material for: Creation and control of a two-dimensional electron liquid at the bare SrTiO3 surface
Source: arXiv:1010.0763 source file (2011-05-08)
Supplement: Supplementary file 1 [file supplementary_info.pdf]

# Supplementary Information for: Creation and control of a two-dimensional electron liquid at the bare $SrTiO_3$ surface

W. Meevasana, P.D.C. King, R.H. He, S.-K. Mo, M. Hashimoto,
A. Tamai, P. Songsiriritthigul, F. Baumberger, and Z.-X. Shen
(Dated: May 8, 2011)

## I. MATERIALS AND METHODS

The measured single crystals are $La_xSr_{1-x}TiO_3$ (Crystal Base Co., Japan) with x = 0.001. The samples are gray in color and partially transparent, confirming their low doping. ARPES data were collected on a Scienta-R4000 analyzer at the Advanced Light Source (ALS), Beamline 10.0.1, with photon energies between 45 - 60 eV and a base pressure of $< 4 \times 10^{-11}$ torr. Additional data, including the valence band spectra shown in Fig. S3, was collected at the Surface and Interface Spectroscopy (SIS) beamline of the Swiss Light Source. All ARPES data was measured with an energy resolution of 6 - 35 meV and an angular resolution of 0.35°. Samples were cleaved at the measurement temperature of T = 20 K along notches defining a (100) plane. This results in flatter surfaces than fracturing or scraping of $SrTiO_3$ as performed previously [1]. Note, however, that the cleaved (100) surface consists of SrO and $TiO_2$ facets. A recent STM study reports flat terraces of $TiO_2$ separated by stepped SrO terminations [2]. The typical morphology of the latter renders it unlikely that the well defined 2DEG states observed here are supported by the SrO terminated surface. Hence, we expect that our ARPES data mostly represent the $TiO_2$ surface. A similar assignment was suggested earlier by Airua et al. [1].

The intensity $I$ of the UV radiation is estimated from the measured photocurrent $I_p$ from the sample and the exposed area of 150 $\mu$m (horizontal) times 60 - 100 $\mu$m (vertical, depending on beamline settings). The clear (1 x 1) low-energy-electron-diffraction (LEED) patterns shown in Fig. S1, which were taken after the ARPES measurements, indicate a well-ordered surface devoid of any reconstructions.

To probe the influence of the surface 2DEG formation on the transport properties of $SrTiO_3$, we also measured the resistivity at the surface of undoped $SrTiO_3$ both before and after UV irradiation. The measurements were performed at room temperature in vacuum (pressure $< 1 \times 10^{-8}$ mbar, on Beamline 3.2a of the Synchrotron Light Research Institute (SLRI), Thailand) using a Keithley electrometer. After irradiation with similar doses as in the ARPES work we observed a drop in resistivity by a factor of $\approx 20$, consistent with the formation of a conducting 2DEG.

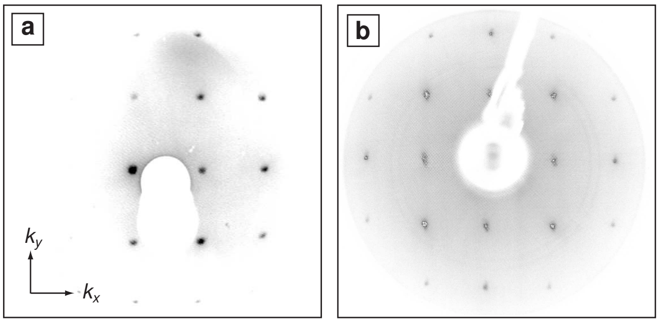


FIG. S1: Low energy electron diffraction (LEED) patterns of $La_xSr_{1-x}TiO_3$ showing clear c(1x1) patterns with no sign of surface reconstruction. a) LEED pattern from a $x = 0.001$ sample, taken at $T = 20$ K immediately after the ARPES measurements. b) A similar diffraction pattern is observed in a $x = 0.05$ sample with much higher carrier density.

### A. 2D character of the observed bands

We confirmed the absence of significant band dispersion along the direction perpendicular to the surface ($k_z$) by varying the incident photon energy. Fig. S2a-e show dispersion plots of the 2DEG states for photon energies ranging from 45 eV to 65 eV corresponding to estimated $k_z$ values of 2.6 - 3.8$\pi/a$. The Fermi momenta $k_F$ extracted from this data (Fig. S2f) are constant within our experimental accuracy, indicating a highly two-dimensional (2D) character of the observed bands. The in-plane parabolic $E(k)$ dispersion relation with no dispersion along $k_z$, as directly measured here, is the defining property of a 2DEG.

### B. Changes in the valence band spectra with UV light exposure

We have shown in the main text that the surface charge density can be modified by increasing the irradiation dose to which the surface is exposed. Here, we discuss the corresponding changes in the oxygen valance band in more detail.

Fig. S3 shows angle-integrated photoemission (AIPES) valence band spectra for different exposures to dim UV light ($I_p$ = 0.38 nA). At $t = 0$ (black line), the spectrum shows clear oxygen $2p$ (O$2p$) states between $\sim 3 - 9$ eV, and no significant spectral weight in the band gap ($0 - 3$ eV). As the exposure time increases, the spectral weight of the O$2p$ state decreases slightly and its

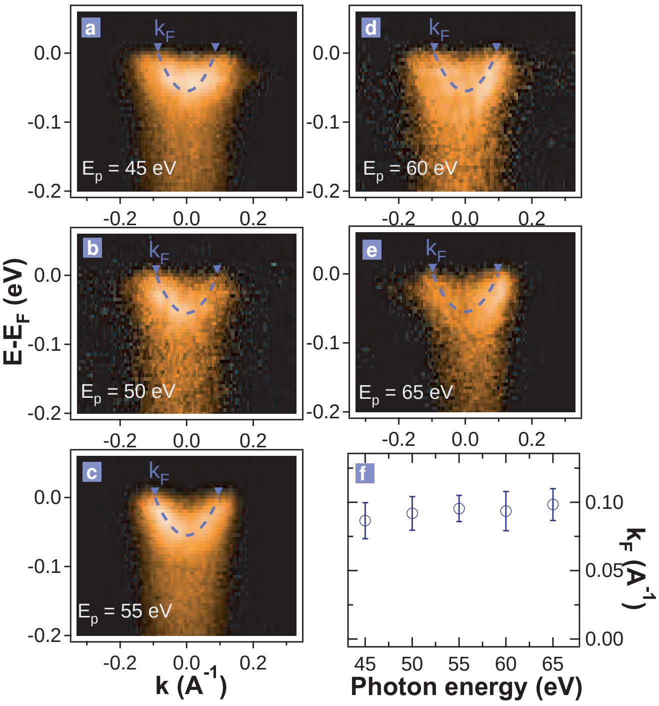


FIG. S2: Photon energy dependence of ARPES data indicating negligible $k_z$ dispersion. a)-e) show ARPES data measured with low photon flux at various photon energies $E_p$ indicated in the figure. The sample has been exposed to $\sim$ 60 J/cm$^2$ prior to the first measurements shown in panel a). f) summarizes the Fermi momenta $k_F$ extracted from a)-e). The range of photon energies corresponds to estimated $k_z$ values from 2.6 - 3.8$\pi/a$.

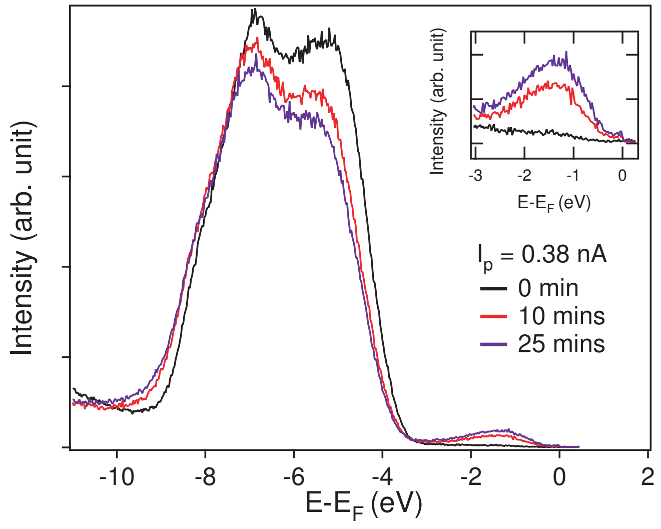


FIG. S3: Evolution of the valance band (VB) spectra of $SrTiO_3$ from the pristine cleaved surface to the exposed surface. The inset shows the evolution of the in-gap state with increasing exposure to UV light.

leading edge shifts to higher binding energy. This indicates an increase in the valence band maximum to surface Fermi level separation, consistent with a downward band bending and development of a 2DEG at the surface, as discussed in the main text. We note that a recent study on semiconductor surface 2DEGs [3] indicates that the valence and conduction band bendings do not need to be equal, due to many-body interactions within the surface 2DEG. Indeed, the valence band bending puts a lower limit on the amount of downward bending of the conduction band, consistent with the situation we observe here.

Together with the valence band shift we also observe a broad in-gap state developing at a binding energy of $\sim$ 1.3 eV. Following earlier studies, we consider that this state is most likely associated with oxygen vacancies at the surface [1], which we attribute as the origin of the donor defect states inducing the 2DEG which we observe following UV-irradiation.

We also note, however, that hydrogen can act as a donor in perovskite titanate compounds [4, 5], providing a second possible source of the microscopic donor surface states. We experimentally confirmed that exposure to the residual gases from the vacuum alone was not sufficient to induce the 2DEG states by performing AIPES measurements at different positions on the same sample. Since the light spot size is much smaller than the sample this allows us to separate the influence of residual gas and exposure to UV light. Moving to a previously unexposed area after performing the measurements described above, we find that the valence band fully recovers to the $t = 0$ spectrum from Fig. S3. Only following sufficient UV light exposure, the in-gap state develops again and the valence band shifts to higher binding energy. This confirms that UV light exposure is crucial for the development of the 2DEG states. However, as $SrTiO_3$ is known to promote photocatalysis [6], we cannot exclude that, in the presence of residual water vapor in the vacuum, the exposure to UV light could generate atomic hydrogen at the surface. Hydrogen adsorption at the surface could also give rise to the in-gap defect peak that we observe [4], and we cannot distinguish between this and oxygen vacancies with our experimental measurements. This should therefore be the subject of future investigations. However, our analysis and conclusions presented in the main manuscript are not sensitive to the exact microscopic nature of the defects causing the charge accumulation.

## C. Calculations

The downward bending of the conduction band and dispersions of the 2DEG states are described by a non-parabolic coupled Poisson-Schröodinger scheme, described in detail elsewhere [7]. In the calculations, the downward conduction-band bending is -0.7 eV at the surface, the bulk band gap is 3.3 eV, the bulk electron concentration is $1.8\times10^{19}$ cm$^3$ and the effective mass is set to

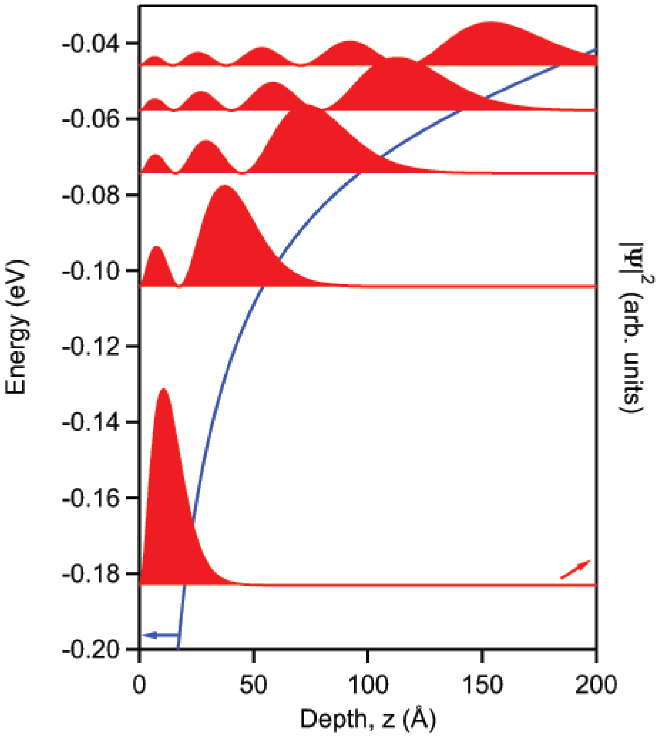


FIG. S4: Poisson-Schrödinger calculations of the surface-normal component of the eigen-functions (red) of the quantized states within the potential well caused by the downward band bending (blue). The modulus squared of the eigen-functions are shown, vertically offset to the respective subband binding energy within the well.

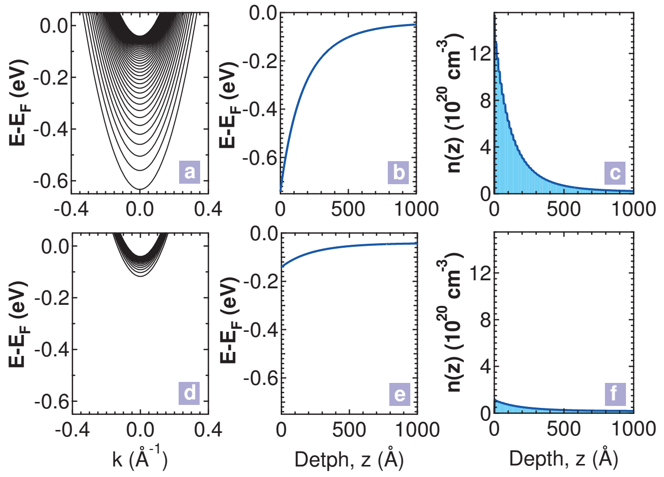


FIG. S5: Calculations of quantized states with the increased charge density wide-spread in sample depth. Both calculations are performed with a more three-dimensional (3D) character of the charge density increase in the vicinity of the surface, with the depth characterizing the band bending increased by a factor of approximately 10 relative to the calculation shown in Fig. 3 of the main manuscript. In (a)-(c), the conduction band bending is set to -0.7eV at the surface, as in Fig. 3, while in (d)-(f), the conduction band bending is set to -0.1eV. The calculations yield many quantized states as shown in (a) and (d). The band bendings as a function of sample depth are shown in (b) and (e), while the corresponding 3D charge density variations are shown in (c) and (f).

$0.6m_e$. The bulk dielectric constant is set to 8000 at T= 20K and zero-field and an electric-field dependent susceptibility model [8] is incorporated. An iterative approach is used to ensure self-consistency between the dielectric constant and band bending potential variation as a function of depth below the surface.

The result of realistic calculations is shown in Fig. 3 of the main manuscript. We find a rapid downward band bending, causing the conduction-band states to become quantized into a ladder of subbands. The surface-normal component of their wave functions are shown in Fig. S4. The wave function of the lowest subband is peaked less than 3 unit cells from the surface, while the probability density of the higher-lying subbands progressively extend deeper in the bulk. Together, these lead to an increase in charge density, strongly peaked in a narrow region ($\sim$10 Å) close to the surface. This narrow spatial extent of the increased charge density, resulting from the strongly confined nature of particularly the lowest subband wave function, strongly supports the two-dimensional character of the 2DEG states observed from ARPES.

To further verify such a strongly confined nature of the observed electronic states, we have performed additional calculations where we artificially force the band bending to occur over larger distances. Consequently, the increased electron density approaching the surface is spread further into the bulk (that is, the system becomes more three-dimensional), as shown in Fig. S5. For the calculation in Fig. S5a-c, the conduction-band bending is kept at -0.7 eV (as in Fig. 3 of the main manuscript) but the effective width is extended by a factor of approximately 10. The electronic states in such a situation rapidly approach a continuum limit, resulting in many subbands and a large sheet density of $1.9 \times 10^{15}$ cm$^{-2}$ which is much higher than the value extracted from the ARPES data. An order-of-magnitude lower sheet density, much closer to the experimentally-observed value, can be obtained by reducing the magnitude of the band banding to 0.1 eV, as shown in Fig. S5d-f. However, the resulting calculations still show large discrepancies with the measured ARPES: the calculated 2DEG states are shallower than the measured states by approximately a factor of two, while there are still many more subbands predicted than are observed. Further, this degree of band bending is unreasonably small, being smaller than the shift of the valence band seen in Fig. S3 which puts a lower limit on the amount of conduction band bending. These calculations, therefore, confirm that a more three-dimensional character of the electron gas formed at the surface of $SrTiO_3$ following UV-irradiation than considered in the main manuscript is inconsistent with the electronic states that we directly observe from ARPES, thus further validating their two-dimensional nature.

[1] Aiura, Y. *et al.* Photoemission study of the metallic state of lightly electron-doped $SrTiO_3$. *Surf. Sci.* **515**, 61 (2002), *and references therein.*

[2] Guisinger, N. P. *et al.* Nanometer-Scale Striped Surface Terminations on Fractured $SrTiO_3$ Surfaces. *ACS Nano.* **3**, 4132 (2009).

[3] King, P. D. C. *et al.* Surface band gap narrowing in quantized electron accumulation layers. *Phys. Rev. Lett.* **104**, 256803 (2010).

[4] Lin, F. *et al.* Hydrogen-induced metallicity of $SrTiO_3$ (001) surfaces: A density functional theory study *Phys. Rev. B* **79**, 035311 (2009), *and references therein.*

[5] Xiong, K., Robertson, J. & Clark, S. J. Behavior of hydrogen in wide band gap oxides. *J. Appl. Phys.* **102**, 083710 (2007).

[6] Miyauchi, M., Takashio, M., & Tobimatsu, H. Photocatalytic Activity of SrTiO3 Codoped with Nitrogen and Lanthanum under Visible Light Illumination *Langmuir* **20**, 232-236 (2004).

[7] King, P. D. C., Veal, T. D. & McConville, C. F. Nonparabolic coupled Poisson-Schrodinger solutions for quantized electron accumulation layers: Band bending, charge profile, and subbands at InN surfaces. *Phys. Rev. B* **77**, 125305 (2008).

[8] Copie, O. *et al.* Towards Two-Dimensional Metallic Behavior at $LaAlO_3/SrTiO_3$ Interfaces. *Phys. Rev. Lett.* **102**, 216804 (2009).
